# Supplementary material for: Nonthermal hydrogen loss at Mars: Contributions of photochemical mechanisms to escape and identification of key processes
Source: arXiv:2308.13105 source file (2023-08-24)
Supplement: Supplementary file 1 [file Gregory+et_al_SI.pdf]

# Supporting Information for “Nonthermal hydrogen loss at Mars: Contributions of photochemical mechanisms to escape and identification of key processes”

Bethan S. Gregory<sup>1</sup>, Michael S. Chaffin<sup>1</sup>, Rodney D. Elliott<sup>1</sup>, Justin

Deighan<sup>1</sup>, Hannes Gröller<sup>2</sup>, and Eryn Cangi<sup>1</sup>

<sup>1</sup>Laboratory for Atmospheric and Space Physics, University of Colorado Boulder, Boulder, Colorado, USA

<sup>2</sup>Lunar and Planetary Laboratory, University of Arizona, Tucson, Arizona, USA

## Contents of this file

1. Profiles of the fraction of H produced above escape energy (charge exchange mechanisms only)
2. Caption for Table S1 (Excel file uploaded separately)
3. Figures S1 to S4

**Profiles of fraction of H produced above escape energy (charge exchange mechanisms only)** Altitude profiles describing the fraction of hydrogen atoms that are produced above the escape energy for the charge exchange reactions between hydrogen ions and O (R8) and H (R11) are shown in Figure S1c. To obtain the fraction of H produced above the escape energy at altitude  $z$ ,  $q(z)$ , we integrate under the Maxwell-Boltzmann

---

energy distribution for the ion temperature,  $T_i(z)$ :

$$q(z) = \int_{0.13-E_I}^{\infty} 2\sqrt{\frac{E}{\pi}} \left( \frac{1}{k_B T_i(z)} \right)^{3/2} e^{-E/k_B T_i(z)} dE \quad (1)$$

where  $E$  is the energy and  $k_B$  is the Boltzmann constant. We integrate between  $0.13 \text{ eV} - E_I$  and infinity, where  $0.13 \text{ eV}$  is the escape energy of a hydrogen atom at  $80 \text{ km}$  and  $E_I$  is the difference in ionization potential between hydrogen and the original neutral atom. For resonant charge exchange,  $E_I$  is zero, and for charge exchange between oxygen and  $\text{H}^+$ ,  $E_I$  is  $-0.019 \text{ eV}$ . Note that this is an upper limit for  $q$ , as we assume that all the kinetic energy of the initial ion, except that required to ionize the O in R8, is kept by the H when it is neutralized.

## References

- Fox, J. L. (2015). The chemistry of protonated species in the martian ionosphere. *Icarus*, 252, 366-392. doi: <https://doi.org/10.1016/j.icarus.2015.01.010>
- Fox, J. L., Zhou, P., & Bougher, S. (1996). The Martian thermosphere/ionosphere at high and low solar activities. *Advances in Space Research*, 17(11), 203-218. doi: [https://doi.org/10.1016/0273-1177\(95\)00751-Y](https://doi.org/10.1016/0273-1177(95)00751-Y)
- Shematovich, V. I. (2013). Suprathermal oxygen and hydrogen atoms in the upper Martian atmosphere. *Solar System Research*, 47(6), 437-445. doi: <https://doi.org/10.1134/S0038094613060087>
- Zhang, P., Kharchenko, V., Jamieson, M. J., & Dalgarno, A. (2009). Energy relaxation in collisions of hydrogen and deuterium with oxygen atoms. *Journal of Geophysical Research: Space Physics*, 114(A7). doi: <https://doi.org/10.1029/2009JA014055>

**Table S1 (caption for separate Excel document)** Table showing input and output data for all 47 mechanisms, for both low and high solar activity conditions and for all five escape probability curves. Data include rate coefficients, excess energies, peak production altitudes, total column production rates, and escape fluxes. Columns Q and AJ show the escape flux calculated using the most appropriate escape probability curve.

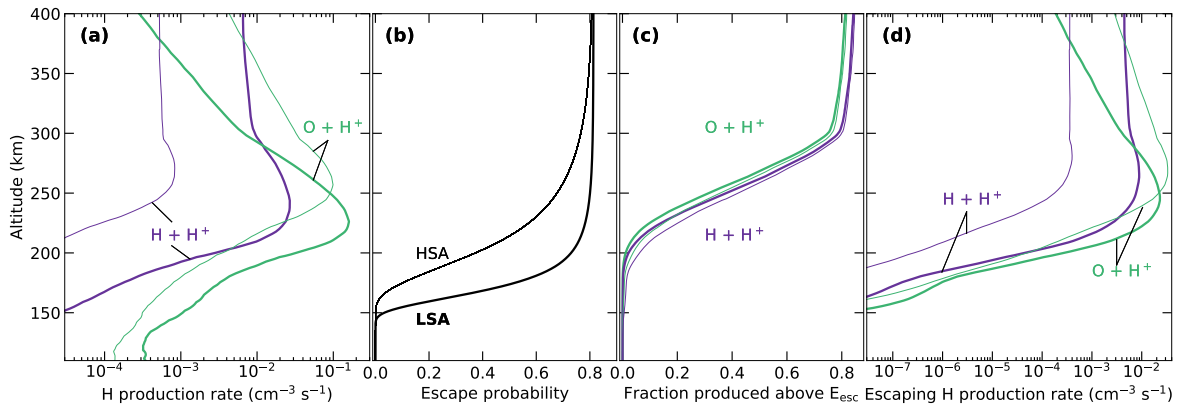

**Figure S1.** Method for estimating escape fluxes for the two charge exchange reactions only. Production rate profiles (a) are multiplied by escape probability profiles (b) and profiles of the fraction of particles produced above the escape energy (c) to obtain profiles of the production rate of escaping hot H (d). Profiles for resonant charge exchange (R11) are shown in purple, and those for charge exchange between a neutral oxygen atom and a hydrogen ion (R8) are shown in teal. Panel (b) shows only the escape probability profiles for an initial kinetic energy of 0.2 eV, which is the most appropriate energy to use for these mechanisms. Profiles for low solar activity are shown by thicker lines, and profiles for high solar activity are shown by thinner lines.

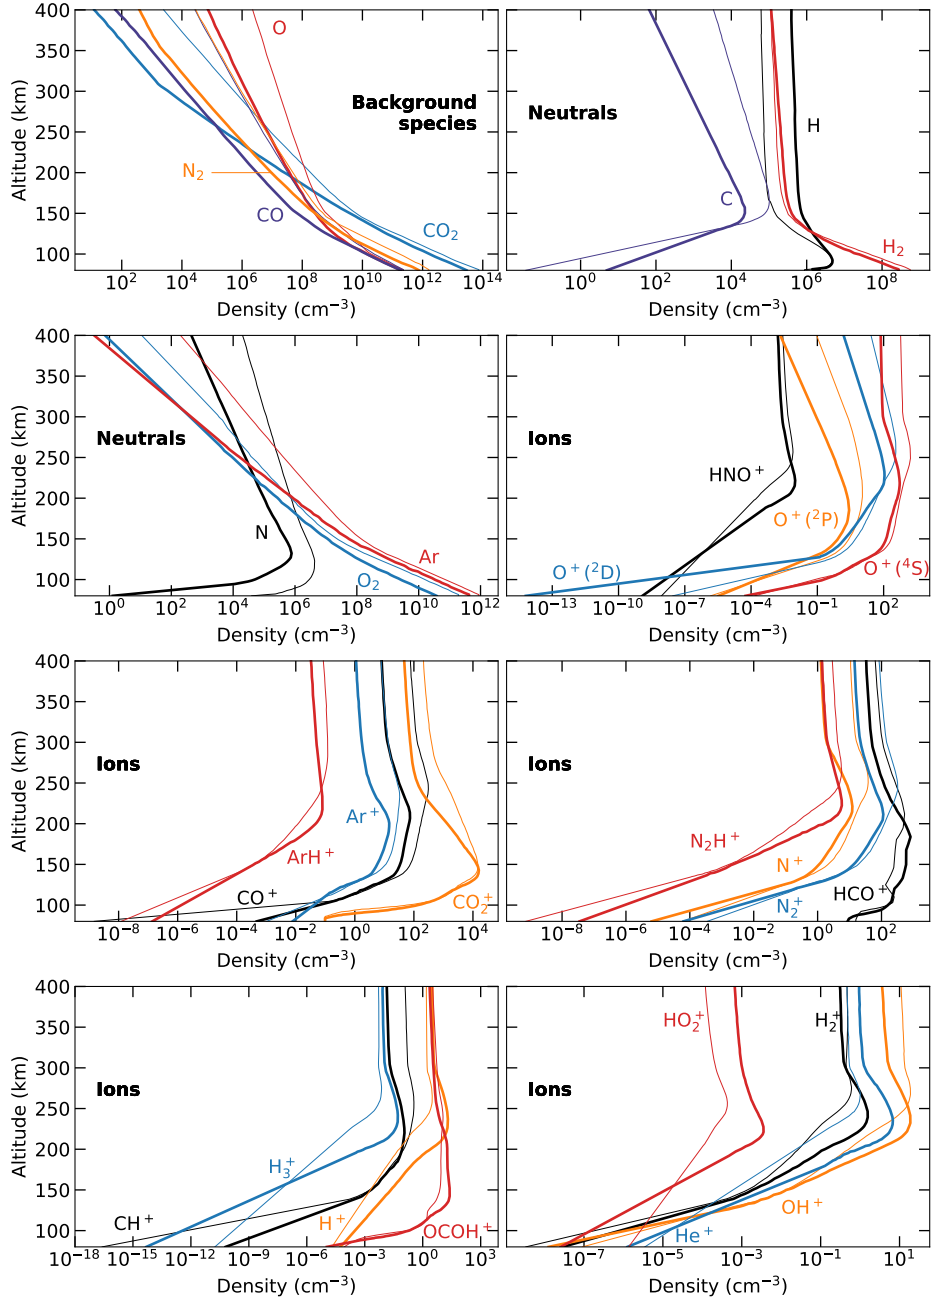

**Figure S2.** Density profiles used, predominantly from Fox (2015). Densities of O<sup>+</sup>(<sup>4</sup>S) are those of O<sup>+</sup>(<sup>2</sup>D) and O<sup>+</sup>(<sup>2</sup>P) (from Fox et al., 1996) subtracted from those of O<sup>+</sup> (from Fox, 2015). Densities are linearly extrapolated in altitude–log(density) space to give complete profiles between 80 km and 400 km. Thick lines are for low solar activity conditions, and thin lines are for high solar activity conditions.

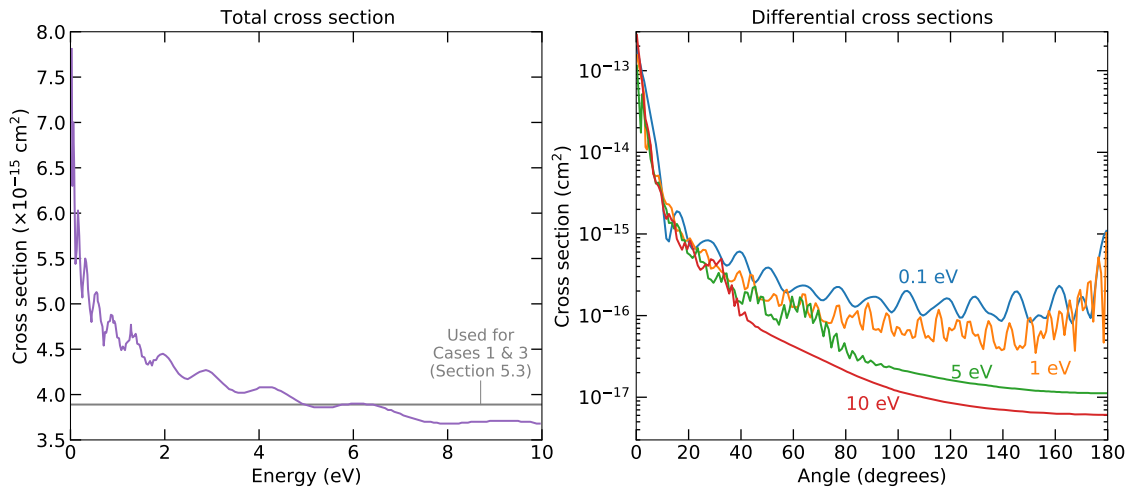

**Figure S3.** Total (a) and differential (b) cross sections used in the model, from Zhang et al. (2009). Differential cross sections have been log-linearly extrapolated beyond  $10^{-13} \text{ cm}^2$  (for angles less than  $\sim 2^\circ$ ). The total cross section, constant with energy, that was used in the Case 1 and 3 experiments described in Section 5.3 and Table 3 is shown in gray in panel (a).

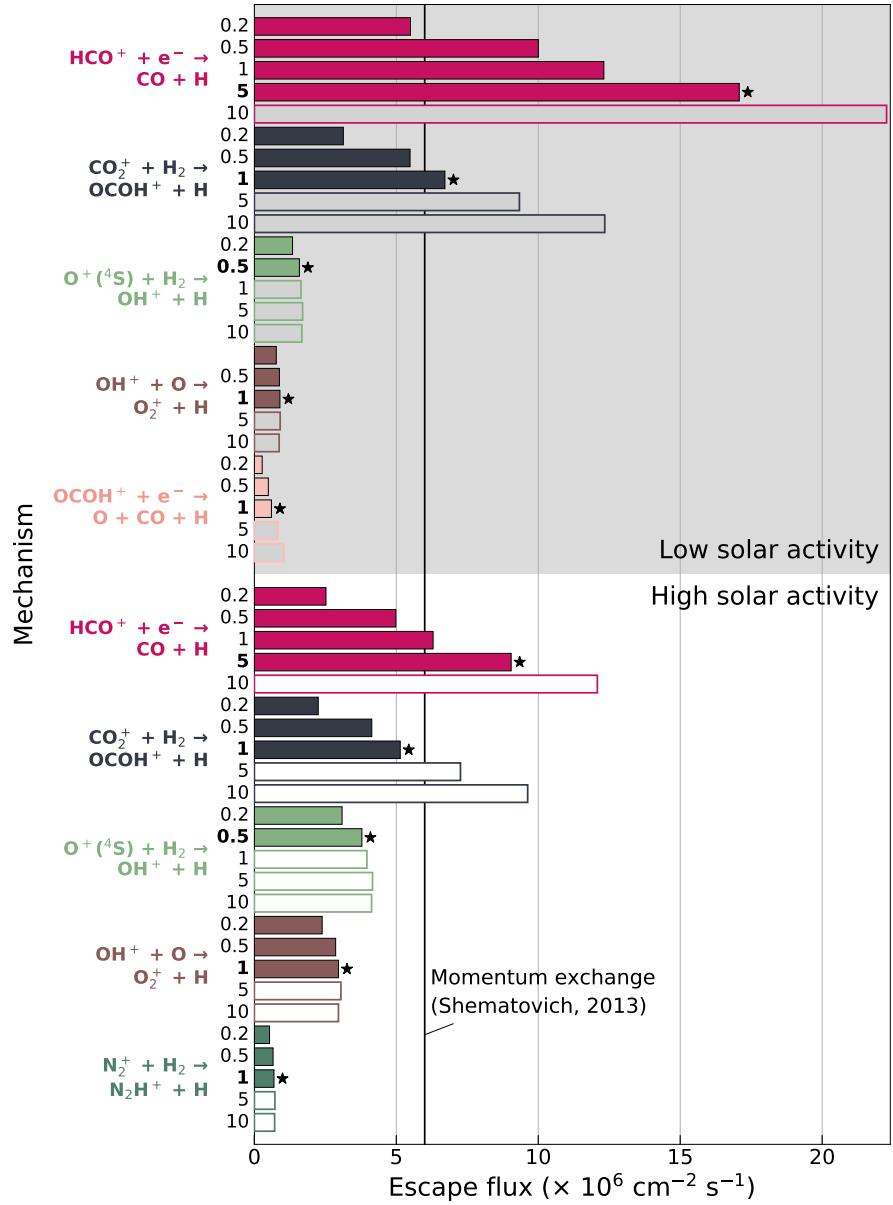

**Figure S4.** Escape fluxes from the top five mechanisms, assuming five different initial particle energies. Fluxes are shown for both low (upper half of plot, gray shading) and high (lower half of plot, no shading) solar activity conditions. Initial particle energies are shown along the vertical axis in units of eV. The flux we consider most likely based on the excess energy of each reaction is marked by the star symbol and the energy label in bold font; this is also the highest of the five energies that can be used for each mechanism. Note that kinetic energies marked by unfilled bars are impossible; we plot them only to demonstrate broad trends in the dependence of escape on energy. Mechanisms that peak lower in the atmosphere have a larger dependence on the selected cross sections. For comparison, the H escape flux via momentum exchange with hot oxygen atoms, calculated by Shematovich (2013), is indicated by the black vertical line.
